# Supplementary material for: CycleINR: Cycle Implicit Neural Representation for Arbitrary-Scale Volumetric Super-Resolution of Medical Data
Source: arXiv:2404.04878 source file (2024-04-07)
Supplement: Supplementary file 1 [file X_suppl.tex]

\clearpage
\setcounter{page}{1}
\maketitlesupplementary
% \section{Supplemental Material }
% \label{sec:supp}

% Deadline: 27 Nov 4:00pm China time
% Set section number to alphabet

\setcounter{section}{0}

\section{Implementation Details}
The proposed CycleINR method was trained using a single Nvidia Tesla V100 GPU, requiring approximately 48 hours to complete 3000 epochs of training. The balancing factor $\lambda$ in Equation \ref{eq11} for the INR fitting loss and cycle-consistent loss is chosen empirically. The code will be made publicly available. 

\section{Visualized efficacy of LAM}
The visualized efficacy of the proposed cycle-consistent loss (CCL) can be demonstrated in Figure \ref{fig3} in the main text, where the phenomena of over-smoothing in the newly generated images and the resultant appearance of horizontal lines in the coronal and sagittal views have been significantly mitigated. 
% Figure \ref{fig5} shows the visualized impact of the proposed local attention mechanism (LAM). The figure displays the error images, which are computed by subtracting the ground truth image from the generated super-resolution images. This figure demonstrates that the incorporation of the local attention mechanism contributes to the preservation of image edges and the retention of fine details. 
Figure \ref{fig5} illustrates the visual impact of the introduced local attention mechanism (LAM), depicted through error images obtained by the subtraction of the ground truth from the generated super-resolution images. The representation underscores the local attention mechanism's role in edge preservation and the maintenance of image detail.
\begin{figure}[!h]
    \includegraphics[width=0.48\textwidth]{fig/02-5.pdf} 
    \caption{Visualized demonstration of LAM on edge and image detail preserving. The display window for the error image  is [-200Hu, 200Hu].}
    \label{fig5}
\end{figure}

\section{SNLI Metric Scatterplot}
Figure \ref{fig6} shows a sample-by-sample SNLI metric scatterplot of different methods to quantitatively show the advantage of CycleINR method on reducing slice-wise noise level inconsistency compared to other three deep learning-based methods. 
\begin{figure}[!h]
    \includegraphics[width=0.48\textwidth]{fig/02-8.pdf} 
    \vspace{-0.4cm}
    \caption{Sample-by-sample SNLI metric scatterplot of different methods on the chest CT dataset to show that the proposed CycleINR method can significantly reduce the slice-wise noise level incosistency compared to other three deep learning-based methods.}
    \vspace{-0.4cm}
    \label{fig6}
\end{figure}

\section{Arbitrary-scale Super-resolution of CycleINR}
Figure \ref{fig4} illustrates the visualization results of the proposed CycleINR method at different Z-spacing scales using one single trained model, highlighting the capability of CycleINR for achieving volumetric super-resolution at arbitrary scales without additional training. It is noteworthy that increasing the resolution along the z-axis leads to enhanced overall image quality. For example, the bone structures that were previously fragmented at 5mm slice thickness can be effectively reconstructed. The previously disconnected structures resulting from poor z-axis resolution can be seamlessly connected and the jagged artifacts have also been alleviated with the enhancement of CycleINR. The overall clarity of the image has also been significantly improved with the increase in the super-resolution scale.

\begin{figure*}[!t]
    \includegraphics[width=1.0\textwidth]{fig/02-4.pdf}

    \caption{Super-resolution results under different scales using only one single trained CycleINR model. Zoom in to obtain a better visual experience. In the first and last rows, it is evident that as the Z-axis super-resolution scale increases, bone structures initially fragmented at 5mm slice thickness can be effectively reconstructed. In the second row, we can see that the jagged artifacts along the liver edge have also been significantly alleviated with the increase of the Z-axis super-resolution scale. In addition, the third and fourth rows demonstrate that structures that were previously disconnected due to poor z-axis resolution can be reconnected after the enhancement of the z-axis resolution.}
    \label{fig4}
\end{figure*}

% % 
% Having the supplementary compiled together with the main paper means that:
% % 
% \begin{itemize}
% \item The supplementary can back-reference sections of the main paper, for example, we can refer to \cref{sec:intro};
% \item The main paper can forward reference sub-sections within the supplementary explicitly (e.g. referring to a particular experiment); 
% \item When submitted to arXiv, the supplementary will already included at the end of the paper.
% \end{itemize}
% % 
% To split the supplementary pages from the main paper, you can use \href{https://support.apple.com/en-ca/guide/preview/prvw11793/mac#:~:text=Delete%20a%20page%20from%20a,or%20choose%20Edit%20%3E%20Delete).}{Preview (on macOS)}, \href{https://www.adobe.com/acrobat/how-to/delete-pages-from-pdf.html#:~:text=Choose%20%E2%80%9CTools%E2%80%9D%20%3E%20%E2%80%9COrganize,or%20pages%20from%20the%20file.}{Adobe Acrobat} (on all OSs), as well as \href{https://superuser.com/questions/517986/is-it-possible-to-delete-some-pages-of-a-pdf-document}{command line tools}.
